# Supplementary material for: A Typology of Decision-Making Tasks for Visualization
Source: arXiv:2404.08812 source file (2026-02-16)
Supplement: Supplementary file 1 [file SupplementalMaterials.tex]

\newpage

\section{Supplemental Materials}
\label{sec:supplementals}
\subsection{Quotes Supporting the Design Goals for a Decision Task Typology}
%[itemsep=0pt, parsep=3pt, leftmargin=*]
\begin{enumerate}[label=\textbf{G\arabic*}]
    \item \label{goal:iteration} \textbf{Iteration}: Given that decision-making processes in visualization often involve cycles and iterations, our typology should incorporate a mechanism to express such iterative patterns.
    \begin{itemize}[leftmargin=*]
        \item ``\textit{By working with the domain experts, we constructed a three-stage iterative workflow for analyzing and improving bus networks}''\cite{weng2021towardsbetterbus}
        \item ``\textit{Planners, stakeholders, and development team members work together in planning their project using ReleasePlanner; the iterative standard planning procedures include...}''\cite{aseniero2015stratos}
    \end{itemize}
    \item \label{goal:hierarchical} \textbf{Hierarchical structure}: Decisions are intricate and can be deconstructed into subtasks, necessitating the ability of our typology to capture these hierarchical relationships.
    \begin{itemize}[leftmargin=*]
        \item ``\textit{Our final design improved the layout and probability encoding of the hierarchical-oriented choices.}''\cite{guo2019uncertaintyandalternatives}
        \item ``\textit{We present two design lessons we have learned while developing BNVA. First, hierarchical exploration is mandatory for complex data like bus networks. [...] In this study, we employed a hierarchical exploration approach to dissect a network with multiple coordinated views from the overview to the details and provide visual hints for the users to drill down in the dataset and find interesting patterns.}''\cite{weng2021towardsbetterbus}
    \end{itemize}
    \item \label{goal:process-centric} \textbf{Process-centric approach}: Our typology should focus on delineating the sequence of decisions users encounter, rather than merely representing data-processing flow or interaction order typically outlined in task lists and design requirements of application papers and design studies.
    \begin{itemize}[leftmargin=*]
        \item ``\textit{Using a laboratory model, the authors have investigated various possible methods for breach closure, utilizing procedures such as single-and multi-barrier embankments with different ways of positioning sandbags. [...] We have identified 7 major phases that led to the final solution.}''\cite{waser2010worldlines}
        \item ``\textit{...capturing metadata of the visual exploration process is a key component of the analysis process. Our history tree visualization is able to record users’ decisions and allow them to compare, modify and insert new decisions.}''\cite{afzal2011decisionsupportforepidemic}
        \item ``\textit{Our approach aims to implement the scenario pool concept as we see it: first, create many plans in the preparation phase; second, quickly pick the most appropriate one in the response phase.}''\cite{waser2014manyplans}
        
    \end{itemize}
    \item \label{goal:data-flexibility} \textbf{Information Processing-Focused}: The decision tasks within our typology should demonstrate flexibility and impartiality towards input and output types, instead emphasizing how information is processed and evaluated.
    \begin{itemize}[leftmargin=*]
         \item ``\textit{The person in charge  [..] %of the defenses 
         has an overview of an area where a disaster can happen, and a number of protection measures available. [...] %Given that there is only a limited amount of time, materials and personnel that can be used, the selection of the measures to be deployed is a difficult task. 
         The goal of our steering environment is to allow the user to experiment with various options, and to do it as intuitively as possible.}''\cite{ribicic2012sketchinguncertainty}
         %\item ``\textit{We have experimented [...] %with this approach 
         %in the area of travel planning and developed a system called SmartClient Travel[...].% which supports this process.It includes tools for need identification, visualization of alternatives, and choosing the most suitable one. [...] The catalog should propose solutions and compare them to alternatives, and thus elicit refinement of the buyer's specifications.}'' \cite{pu2000smartclient}
         \item ``\textit{...only information on a few products is given to the buyers, leaving them wondering what other alternatives are available.}''\cite{weng2018homefinder}
          \item ``\textit{This interactive exploratory tool helps the casual decision-maker quickly choose between various financial portfolio options and view possible outcomes.}''\cite{rudolph2009finvis}
    \end{itemize}
\end{enumerate}

\subsection{Diagrams Created by Our Participants}.
\begin{figure}[ht!]
\centering
  \includegraphics[width=0.9\linewidth]{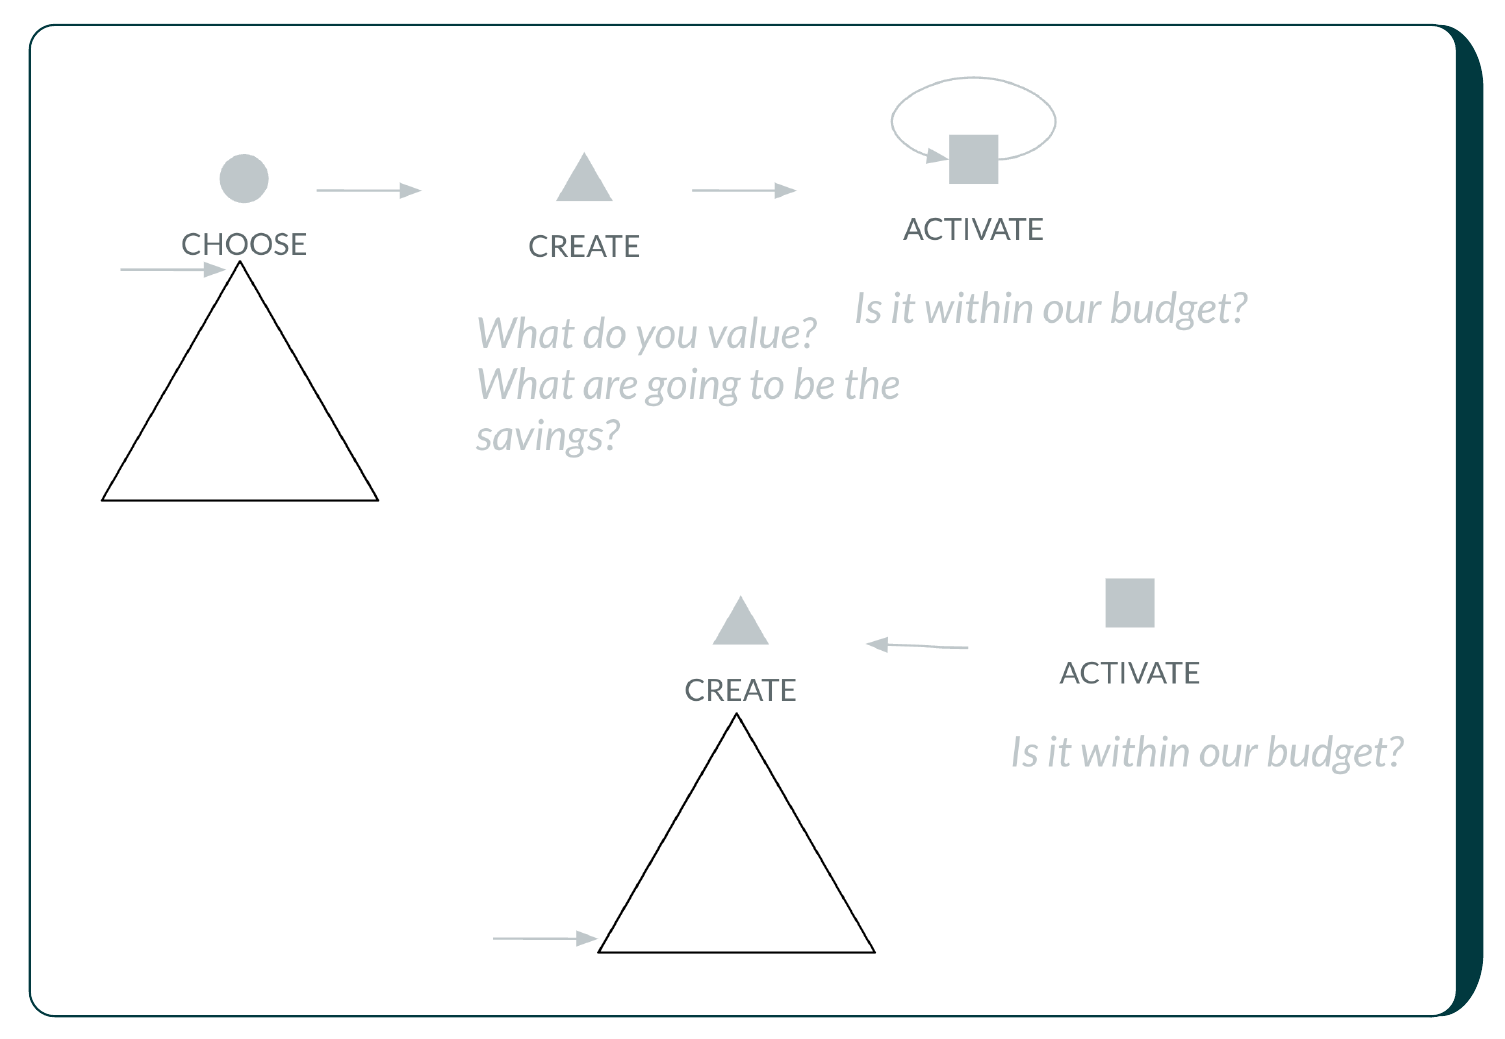}
  \caption{A hierarchy annotation used by one of the participants during the interview study. In this figure, the triangles (and the arrows) indicate the role of a decision-maker in an organization's hierarchy.
  }
  \label{fig:annotation}
\end{figure}

\begin{figure*}[ht!]
    \centering
    \includegraphics[width=\textwidth]{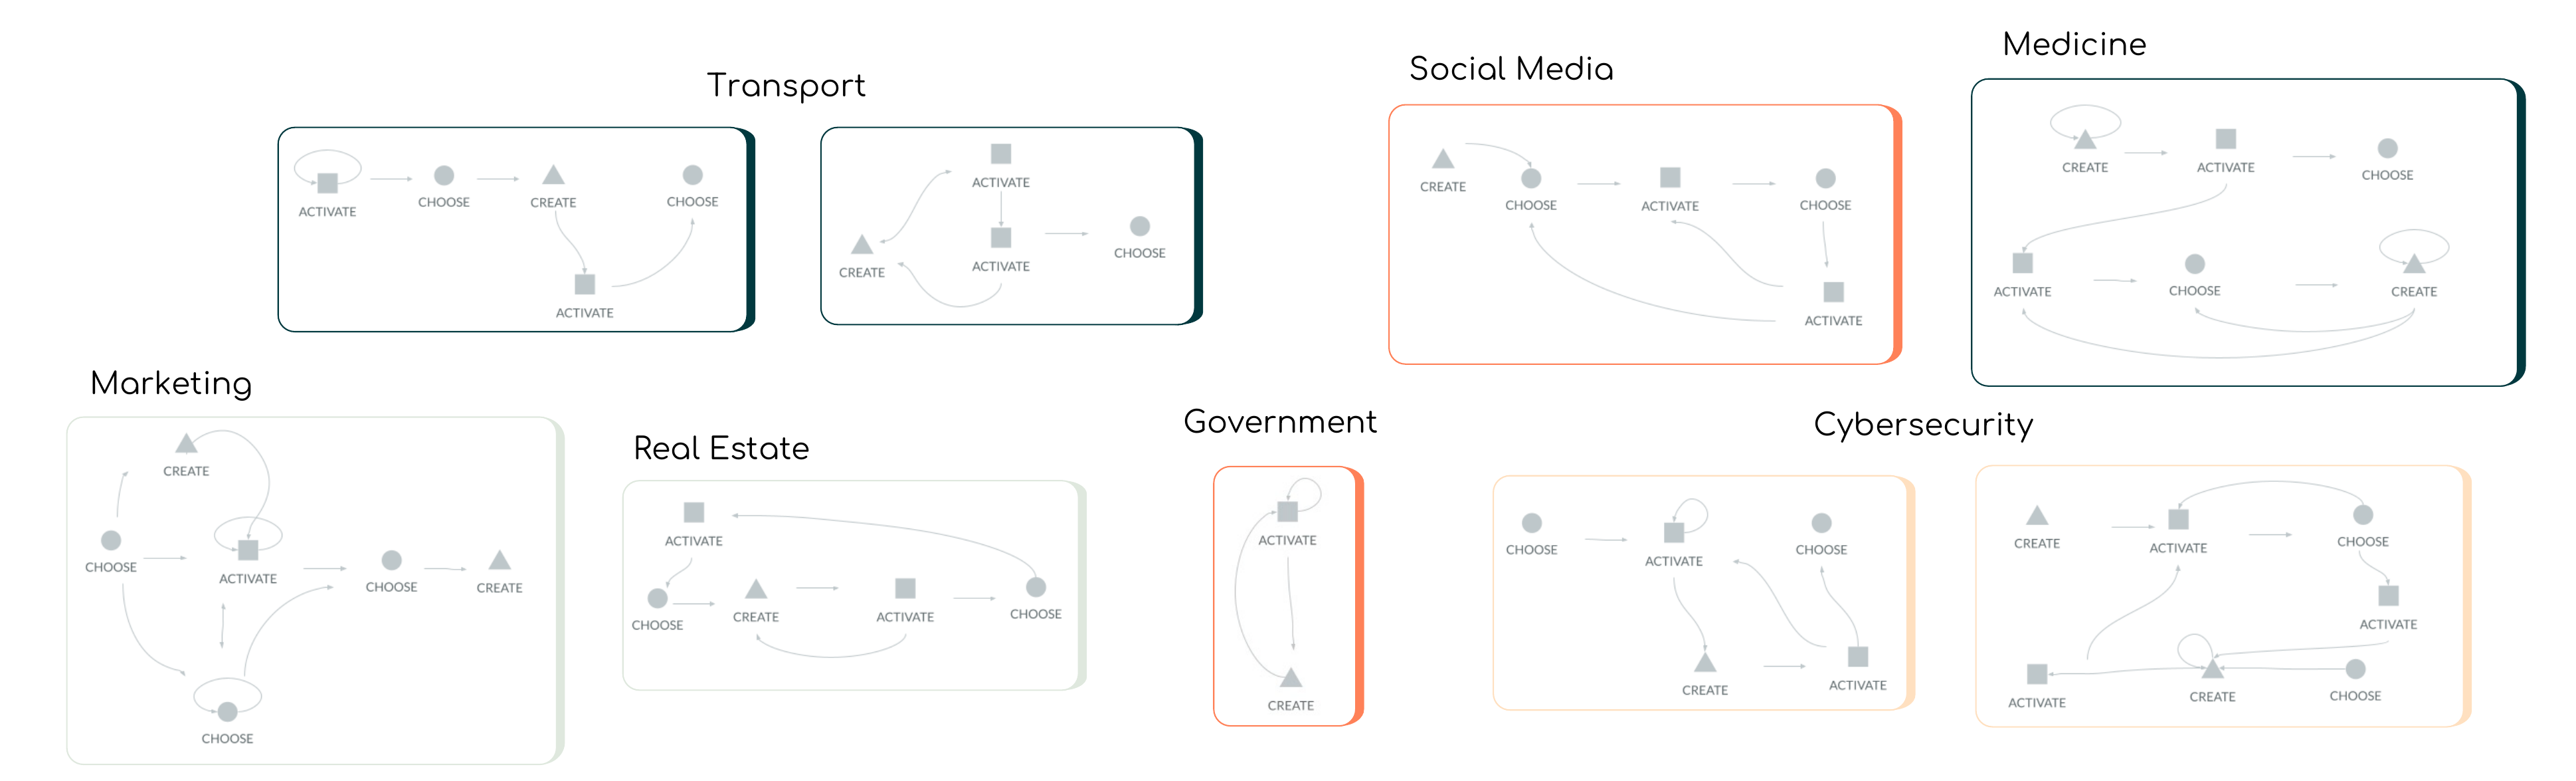}
    \caption{Diagrams created by our participants during the interview study. Texts, labels, and annotations that contain identifiable information have been removed to preserve anonymity. We labeled the diagrams with the domain of application.}
    \label{fig:collage}
\end{figure*}
